# Supplementary material for: Task Weighting in Meta-learning with Trajectory Optimisation
Source: arXiv:2301.01400 source file (2023-01-04)
Supplement: Supplementary file 1 [file gauss_newton_matrix.tex]

\section{Gauss-Newton matrix}
\label{sec:gauss_newton_matrix}
    First, the loss of interest is the sum of losses over many data-points:
    % Let \(\ell_{i}(\mathbf{w}) = \ell(s_{i}, \mathbf{w})\) is the loss on each data point \(s_{i}\). The loss of interest is then defined as:
    \begin{equation}
        L = \sum_{i=1}^{N} \ell (x_{i}, t_{i}, \mathbf{w}),
    \end{equation}
    where:
    \begin{itemize}
        \item \((x_{i}, t_{i})\) is a data-point,
        \item \(\mathbf{w}\) is the parameter of the model of interest, or the weight of a neural network,
        \item \(\ell(.) \in \mathbb{R}\) is the loss function, e.g. MSE or cross-entropy.
    \end{itemize}
    
    Let's define some additional notations as the following:
    \begin{itemize}
        \item \(\mathbf{f}(x_{i}, \mathbf{w}) \in \mathbb{R}^{C}\) is the pre-nonlinearity output of the neural network at the final layer that has \(C\) hidden units,
        \item \(\sigma\left[ \mathbf{f}\left(x_{i}, \mathbf{w}\right) \right] \in \mathbb{R}^{C}\) is the activation output at the final layer. For example, in regression, \(\sigma(z) = z\) is the identity function, or in logistic regression, \(\sigma(.)\) is the sigmoid function, while in multi-class classification, \(\sigma(.)\) is the softmax function,
    \end{itemize}
    
    Second, each loss function of interest can be rewritten as:
    \begin{equation}
        \begin{aligned}[b]
            L & = \sum_{i=1}^{N} \ell \left[ \sigma \left( \mathbf{f}(x_{i}, \mathbf{w}) \right)\right].
        \end{aligned}
    \end{equation}
    In the following, the target \(t_{i}\) is omitted to make the notation uncluttered.
    
    An element of the Hessian matrix can then be written as:
    \begin{equation}
    \begin{aligned}[b]
        \mathbf{H}_{jk} & = \pdv{}{\mathbf{w}_{k}} \left( \pdv{L}{\mathbf{w}_{j}} \right) = \pdv{}{\mathbf{w}_{k}} \left( \sum_{i=1}^{N} \pdv{\ell \left[ \sigma \left( \mathbf{f}(x_{i}, \mathbf{w}) \right)\right]}{\mathbf{w}_{j}} \right) \\
        & = \pdv{}{\mathbf{w}_{k}} \left( \sum_{i=1}^{N} \sum_{c=1}^{C} \pdv{\ell \left[ \sigma \left( \mathbf{f}(x_{i}, \mathbf{w}) \right)\right]}{\mathbf{f}_{c} (x_{i}, \mathbf{w})} \pdv{\mathbf{f}_{c} (x_{i}, \mathbf{w})}{\mathbf{w}_{j}} \right) \quad \text{(chain rule)}\\
        & = \sum_{i=1}^{N} \sum_{c=1}^{C} \pdv{}{\mathbf{w}_{k}} \left( \pdv{\ell \left[ \sigma \left( \mathbf{f}(x_{i}, \mathbf{w}) \right)\right]}{\mathbf{f}_{c} (x_{i}, \mathbf{w})} \pdv{\mathbf{f}_{c} (x_{i}, \mathbf{w})}{\mathbf{w}_{j}} \right).
    \end{aligned}
    \end{equation}
    
    Applying the product rule of derivative gives:
    \begin{equation}
        \mathbf{H}_{jk} = \sum_{i=1}^{N} \sum_{c=1}^{C} \pdv{}{\mathbf{w}_{k}} \left( \pdv{\ell \left[ \sigma \left( \mathbf{f}(x_{i}, \mathbf{w}) \right)\right]}{\mathbf{f}_{c} (x_{i}, \mathbf{w})} \right) \pdv{\mathbf{f}_{c} (x_{i}, \mathbf{w})}{\mathbf{w}_{j}} + \pdv{\ell \left[ \sigma \left( \mathbf{f}(x_{i}, \mathbf{w}) \right)\right]}{\mathbf{f}_{c} (x_{i}, \mathbf{w})} \pdv{\mathbf{f}_{c} (x_{i}, \mathbf{w})}{\mathbf{w}_{j}}{\mathbf{w}_{k}}.
    \end{equation}
    
    Applying the chain rule for the first term gives:
    \begin{equation}
        \begin{aligned}[b]
            \mathbf{H}_{jk} & = \sum_{i=1}^{N} \sum_{c=1}^{C} \left[ \sum_{l=1}^{C} \left( \pdv{\ell \left[ \sigma \left( \mathbf{f}(x_{i}, \mathbf{w}) \right)\right]}{\mathbf{f}_{c} (x_{i}, \mathbf{w})}{\mathbf{f}_{l}(x_{i}, \mathbf{w})} \pdv{\mathbf{f}_{l}(x_{i}, \mathbf{w})}{\mathbf{w}_{k}} \right) \pdv{\mathbf{f}_{c} (x_{i}, \mathbf{w})}{\mathbf{w}_{j}} \right] \\
            & \qquad \qquad \quad + \pdv{\ell \left[ \sigma \left( \mathbf{f}(x_{i}, \mathbf{w}) \right)\right]}{\mathbf{f}_{c} (x_{i}, \mathbf{w})} \pdv{\mathbf{f}_{c} (x_{i}, \mathbf{w})}{\mathbf{w}_{j}}{\mathbf{w}_{k}}.
        \end{aligned}
    \end{equation}
    
    Rearranging gives:
    \begin{equation}
        \begin{aligned}[b]
            \mathbf{H}_{jk} & = \sum_{i=1}^{N} \sum_{c=1}^{C} \pdv{\mathbf{f}_{c} (x_{i}, \mathbf{w})}{\mathbf{w}_{j}} \sum_{l=1}^{C} \pdv{\ell \left[ \sigma \left( \mathbf{f}(x_{i}, \mathbf{w}) \right)\right]}{\mathbf{f}_{c} (x_{i}, \mathbf{w}) }{ \mathbf{f}_{l}(x_{i}, \mathbf{w})} \pdv{\mathbf{f}_{l}(x_{i}, \mathbf{w})}{\mathbf{w}_{k}} \\
            & \quad + \sum_{i=1}^{N} \sum_{c=1}^{C} \underbrace{\pdv{\ell \left[ \sigma \left( \mathbf{f}(x_{i}, \mathbf{w}) \right)\right]}{\mathbf{f}_{c} (x_{i}, \mathbf{w})}}_{\approx 0} \pdv{\mathbf{f}_{c} (x_{i}, \mathbf{w})}{\mathbf{w}_{j} }{\mathbf{w}_{k}}.
        \end{aligned}
    \end{equation}
    
    Near the optimum, the scalar \(\mathbf{f}_{c}\) would be very closed to its target \(\mathbf{t}_{ic}\). Hence, the derivative of the loss w.r.t. \(\mathbf{f}_{c}\) is very small, and we can approximate the Hessian as:
    \begin{equation}
        \mathbf{H}_{jk} \approx \sum_{i=1}^{N} \sum_{c=1}^{C} \pdv{\mathbf{f}_{c} (x_{i}, \mathbf{w})}{\mathbf{w}_{j}} \sum_{l=1}^{C} \pdv{\ell \left[ \sigma \left( \mathbf{f}(x_{i}, \mathbf{w}) \right)\right]}{\mathbf{f}_{c} (x_{i}, \mathbf{w}) }{ \mathbf{f}_{l}(x_{i}, \mathbf{w})} \pdv{\mathbf{f}_{l}(x_{i}, \mathbf{w})}{\mathbf{w}_{k}}.
    \end{equation}
    
    Rewriting this with matrix notation yields a much simpler formulation:
    \begin{equation}
        \mathbf{H} \approx \sum_{i=1}^{N} \mathbf{J}_{fi}^{\top} \mathbf{H}_{\sigma i} \mathbf{J}_{fi},
    \end{equation}
    where:
    \begin{align}
        \mathbf{J}_{fi} & = \nabla_{\mathbf{w}} \mathbf{f}(x_{i}, \mathbf{w}) \in \mathbb{R}^{C \times W} \quad \text{(Jacobian matrix of \textbf{f} w.r.t. \textbf{w})}\\
        \mathbf{H}_{\sigma i} & = \nabla_{\mathbf{f}}^{2} \ell\left[ \sigma \left( \mathbf{f}(x_{i}, \mathbf{w} \right) \right] \in \mathbb{R}^{C \times C} \quad \text{(Hessian of loss w.r.t. \textbf{f})}.
    \end{align}
    
    \begin{remark}[Hessian matrix \(\mathbf{H}_{\sigma}\)]
        The Hessian matrix \(\mathbf{H}_{\sigma}\) can be manually calculated as shown in the following sub-sections.
    \end{remark}
    
    \begin{remark}[Storing Hessian matrix]
        Instead of storing the Hessian matrix \(\mathbf{H}\) with size \({W \times W}\) which needs a large amount of memory, we can store the two matrices \(\{\mathbf{J}_{fi}, \mathbf{H}_{\sigma i}\}_{i=1}^{N}\). This will reduce the amount of memory required. Of course, the trade-off is the increasing of the computation when performing the multiplication to obtain the Hessian matrix \(\mathbf{H}\).
    \end{remark}
    
    \subsection{Mean square error in regression}
        In the regression:
        \begin{itemize}
            \item \(C = 1\)
            \item \(\sigma(.)\) is the identity function
            \item \(\ell(f(x_{i}, \mathbf{w}) = \frac{1}{2} \left( f(x_{i}, \mathbf{w}) - t_{i} \right)^{2}\).
        \end{itemize}
        Hence, \(\mathbf{H}_{\sigma} = \mathbf{I}_{1}\), resulting in \(\mathbf{H} = \sum_{i=1}^{N} \mathbf{J}_{fi}^{\top} \mathbf{J}_{fi}\)%~\citep[Eq.~(5.84)]{bishop2006pattern}.
    
    \subsection{Logistic regression}
        In this case:
        \begin{itemize}
            \item \(C = 1\)
            \item \(\sigma(.)\) is the sigmoid function
            \item \(\ell(\sigma(f(x_{i}, \mathbf{w})) = - t_{i} \ln \sigma \left( f(x_{i}, \mathbf{w}) \right) - (1 - t_{i}) \ln \left( 1 - \sigma \left( f(x_{i}, \mathbf{w}) \right) \right)\).
        \end{itemize}
        The first derivative is expressed as:
        \begin{equation}
            \pdv{\ell(\sigma(f(x_{i}, \mathbf{w}))}{f(x_{i}, \mathbf{w})} = - t_{i} \left( 1 - \sigma \left( f(x_{i}, \mathbf{w}) \right) \right) + (1 - t_{i}) \sigma \left( f(x_{i}, \mathbf{w}) \right) = \sigma \left( f(x_{i}, \mathbf{w}) \right) - t_{i}.
        \end{equation}
        The second derivative is therefore:
        \begin{equation}
            \pdv[2]{\ell(\sigma(f(x_{i}, \mathbf{w}))}{f(x_{i}, \mathbf{w})} = \sigma \left( f(x_{i}, \mathbf{w}) \right) \left[ 1 - \sigma \left( f(x_{i}, \mathbf{w}) \right) \right].
        \end{equation}
        
        Hence:
        \begin{equation}
            \mathbf{H} \approx \sum_{i=1}^{n} \sigma \left( f(x_{i}, \mathbf{w}) \right) \left[ 1 - \sigma \left( f(x_{i}, \mathbf{w}) \right) \right] \mathbf{J}_{fi}^{\top} \mathbf{J}_{fi},
        \end{equation}
        which agrees with the result derived in the literature%~\citep[Eq.~(5.85)]{bishop2006pattern}
    
    \subsection{Cross entropy loss in classification}
        In this case:
        \begin{itemize}
            \item \(\sigma(\mathbf{f})\) is the softmax function,
            \item \(\ell(\sigma(\mathbf{f}(x_{i}, \mathbf{w}))) = -\sum_{c=1}^{C} \mathbf{t}_{ic} \ln \sigma_{c}(\mathbf{f}(x_{i}, \mathbf{w})) = -\mathbf{t}_{i}^{\top} \ln \sigma(\mathbf{f}(x_{i}, \mathbf{w})) \).
        \end{itemize}
        According to the definition of the softmax function:
        \begin{equation}
            \sigma_{c} \left( \mathbf{f} \right) = \frac{\exp(\mathbf{f}_{c})}{\sum_{k=1}^{C} \exp(\mathbf{f}_{k})}.
        \end{equation}
        Hence, the derivative can be written as:
        \begin{equation}
            \pdv{\sigma_{c}(\mathbf{f})}{\mathbf{f}_{c}} = \frac{\exp(\mathbf{f}_{c}) \sum_{k=1}^{C} \exp(\mathbf{f}_{k}) - \exp(2 \mathbf{f}_{c})}{\left[ \sum_{k=1}^{C} \exp(\mathbf{f}_{k}) \right]^{2}} = \sigma_{c}(\mathbf{f}) \left[ 1 - \sigma_{c}(\mathbf{f}) \right],
        \end{equation}
        and
        \begin{equation}
            \pdv{\sigma_{c}(\mathbf{f})}{\mathbf{f}_{k}} = - \sigma_{c}(\mathbf{f}) \sigma_{k}(\mathbf{f}), \forall k \neq j.
        \end{equation}
        
        An element of the Jacobian vector of the loss w.r.t. \(\mathbf{f}\) can be written as:
        \begin{equation}
            \begin{aligned}[b]
                \pdv{\ell(\sigma(\mathbf{f}(x_{i}, \mathbf{w})))}{\mathbf{f}_{c}(x_{i}, \mathbf{w})} & = - \sum_{k=1}^{C} \frac{\mathbf{t}_{ik}}{\sigma_{k}(\mathbf{f})} \pdv{\sigma_{k}(\mathbf{f})}{\mathbf{f}_{c}} \\
                & = - \mathbf{t}_{ic} \left[ 1 - \sigma_{c}(\mathbf{f}) \right] + \sum_{\substack{k=1\\k \neq c}}^{C} \mathbf{t}_{ik} \sigma_{c}(\mathbf{f}) \\
                & = - \mathbf{t}_{ic} + \sigma_{c}(\mathbf{f}) \underbrace{\sum_{k=1}^{C} \mathbf{t}_{ik}}_{1}\\
                & = \sigma_{c}(\mathbf{f}) - \mathbf{t}_{ic}.
            \end{aligned}
        \end{equation}
        
        Hence, the Jacobian vector can be expressed as:
        \begin{equation}
            \nabla_{\mathbf{f}} \ell(\sigma(\mathbf{f}(x_{i}, \mathbf{w}))) = \sigma(\mathbf{f}(x_{i}, \mathbf{w})) - \mathbf{t}_{i}.
        \end{equation}
        
        The Hessian matrix is given as:
        \begin{equation}
            \nabla_{\mathbf{f}}^{2} \ell(\sigma(\mathbf{f}(x_{i}, \mathbf{w}))) = \nabla_{\mathbf{f}} \sigma(\mathbf{f}(x_{i}, \mathbf{w})).
        \end{equation}
        
        Or, in the explicit matrix form:
        \begin{equation}
            \mathbf{H}_{\sigma} = \begin{bmatrix}
            \sigma_{1}(\mathbf{f}) \left[ 1 - \sigma_{1}(\mathbf{f}) \right] & - \sigma_{1}(\mathbf{f}) \sigma_{2}(\mathbf{f}) & - \sigma_{1}(\mathbf{f}) \sigma_{3}(\mathbf{f}) & \ldots & - \sigma_{1}(\mathbf{f}) \sigma_{C}(\mathbf{f})\\
            - \sigma_{2}(\mathbf{f}) \sigma_{1}(\mathbf{f}) & \sigma_{2}(\mathbf{f}) \left[ 1 - \sigma_{2}(\mathbf{f}) \right] & - \sigma_{2}(\mathbf{f}) \sigma_{3}(\mathbf{f}) & \ldots & - \sigma_{2}(\mathbf{f}) \sigma_{C}(\mathbf{f})\\
            \vdots & \vdots & \ddots & \vdots & \vdots\\
            - \sigma_{C}(\mathbf{f}) \sigma_{1}(\mathbf{f}) & - \sigma_{C}(\mathbf{f}) \sigma_{2}(\mathbf{f}) & - \sigma_{C}(\mathbf{f}) \sigma_{3}(\mathbf{f}) & \ldots & \sigma_{C}(\mathbf{f}) \left[ 1 - \sigma_{C}(\mathbf{f}) \right]
            \end{bmatrix}.
        \end{equation}
        
\section{Jacobian vector of the loss w.r.t. \texorpdfstring{\(\mathbf{w}\)}{}}
    Although the Jacobian vector of the loss w.r.t. the network parameter \(\mathbf{w}\) can be calculated separately, we utilise the results of \(\mathbf{J}_{fi}\) to make the implementation efficient. Here, we consider the loss as cross-entropy. In general, an element of the Jacobian vector can be expressed as:
    \begin{equation}
        \pdv{L}{\mathbf{w}_{j}} = \sum_{i=1}^{N} \pdv{\ell\left[ \sigma \left( \mathbf{f}(x_{i}, \mathbf{w} \right) \right]}{\mathbf{w}_{j}} = \sum_{i=1}^{N} \sum_{c=1}^{C} \underbrace{\pdv{\ell \left[ \sigma \left( \mathbf{f}(x_{i}, \mathbf{w}) \right)\right]}{\mathbf{f}_{c} (x_{i}, \mathbf{w})}}_{\sigma_{c}(\mathbf{f}) - \mathbf{t}_{ic}} \underbrace{\pdv{\mathbf{f}_{c} (x_{i}, \mathbf{w})}{\mathbf{w}_{j}}}_{\mathbf{J}_{fi,cj}}.
    \end{equation}
    
    This has a simple form as:
    \begin{equation}
        \mathbf{J}_{j} = \pdv{L}{\mathbf{w}_{j}} = \sum_{i=1}^{N} \sum_{c=1}^{C} \left[ \sigma_{c}(\mathbf{f}) - \mathbf{t}_{ic} \right] \mathbf{J}_{fi,cj}.
    \end{equation}
