# Supplementary material for: Task Weighting in Meta-learning with Trajectory Optimisation
Source: arXiv:2301.01400 source file (2023-01-04)
Supplement: Supplementary file 2 [file protonet_results.tex]

% \section{Additional experimental results for Prototypical Networks}
% \label{sec:protonet_results}

%     \begin{figure}[t]
%         \centering
%         \begin{subfigure}{0.45 \linewidth}
%             \centering
%             \begin{tikzpicture}
%                 \begin{axis}[
%                     height=0.6 \linewidth,
%                     width=0.8 \linewidth,
%                     title={Protonet - mini-ImageNet - train},
%                     % title style={font=\small},
%                     xlabel={Number of training tasks (\(\times 10,000\))},
%                     % xlabel style={font=\small},
%                     % xticklabel style = {font=\small},
%                     xmin=0,
%                     ylabel={Training NLL},
%                     % ylabel style={font=\small},
%                     % yticklabel style = {font=\small},
%                     % ymin=40,
%                     % ymax=42.15,
%                     % restrict x to domain=0:300,
%                     table/col sep=comma,
%                     table/x=x,
%                     table/header=true,
%                     % table/skip rows between index={602}{707},
%                     scale only axis,
%                     legend entries={uniform, exploration, exploitation, TOW},
%                     legend style={draw=none, font=\small},
%                     legend cell align={left},
%                     legend pos=north east
%                 ]
%                     \addplot[mark=none, C0, dashed, very thick] table[y={Training loss_uniform}]{results/protonet_miniImageNet.csv};
%                     \addplot[mark=none, C1, dotted, very thick] table[y={Training loss_exploration}]{results/protonet_miniImageNet.csv};
%                     \addplot[mark=none, C2, dashdotted, very thick] table[y={Training loss_exploitation}]{results/protonet_miniImageNet.csv};
%                     \addplot[mark=none, C3, solid, very thick] table[y={Training loss_tow}]{results/protonet_miniImageNet.csv};
%                 \end{axis}
%             \end{tikzpicture}
%             \caption{}
%             \label{fig:protonet_miniImageNet_training_loss}
%         \end{subfigure}
%         \hfill
%         \begin{subfigure}{0.45 \linewidth}
%             \centering
%             \begin{tikzpicture}%[spy using outlines={circle, magnification=4, size=2cm, connect spies}]
%                 \begin{axis}[
%                     name=ax1,
%                     height=0.6 \linewidth,
%                     width=0.8 \linewidth,
%                     title={Protonet - mini-ImageNet - test},
%                     % title style={font=\small},
%                     xlabel={Number of training tasks (\(\times 10,000\))},
%                     % xlabel = \vphantom{Hello},
%                     % xlabel style={font=\small},
%                     % xticklabel style = {font=\small},
%                     ylabel={Accuracy (\%)},
%                     % ylabel style={font=\small},
%                     % yticklabel style = {font=\small},
%                     ymin=34,
%                     ymax=45.25,
%                     % restrict x to domain=0:300,
%                     table/col sep=comma,
%                     table/x=x,
%                     table/header=true,
%                     % table/skip rows between index={602}{707},
%                     scale only axis
%                     % legend entries={uniform, exploration, exploitation, TOW},
%                     % legend style={draw=none, font=\small},
%                     % legend cell align={left},
%                     % legend pos=north east
%                 ]
%                     \addplot[mark=none, C0, dashed, very thick] table[y={Testing_accuracy_uniform}]{results/protonet_miniImageNet.csv};
%                     \addplot[mark=none, C1, dotted, very thick] table[y={Testing_accuracy_exploration}]{results/protonet_miniImageNet.csv};
%                     \addplot[mark=none, C2, dashdotted, very thick] table[y={Testing_accuracy_exploitation}]{results/protonet_miniImageNet.csv};
%                     \addplot[mark=none, C3, solid, very thick] table[y={Testing_accuracy_tow}]{results/protonet_miniImageNet.csv};
%                     % \spy [black] on (4.5, 2.75) in node at (3.25, 1.25);

%                     % define coordinates at bottom left and top left of rectangle
%                     \coordinate (c1) at (axis cs:270,43);
%                     \coordinate (c2) at (axis cs:295,42);
%                     % draw a rectangle
%                     \draw (c1) rectangle (c2);
%                 \end{axis}

%                 \begin{axis}[
%                     name=ax2,
%                     at={($(ax1.south west)+(2.85cm,0.25cm)$)},
%                     height=0.2 \linewidth,
%                     width = 0.26 \linewidth,
%                     xmin=280,
%                     xmax=290,
%                     ymin=42.55,
%                     ymax=42.75,
%                     ytick={42.55, 42.65, 42.75},
%                     xlabel={},
%                     % ticks=none,
%                     xmajorticks=false,
%                     table/col sep=comma,
%                     table/x=x,
%                     table/header=true,
%                     scale only axis
%                 ]
%                     \addplot[mark=none, C0, dashed, very thick, domain=280:290] table[y={Testing_accuracy_uniform}]{results/protonet_miniImageNet.csv};
%                     \addplot[mark=none, C1, dotted, very thick, domain=280:290] table[y={Testing_accuracy_exploration}]{results/protonet_miniImageNet.csv};
%                     \addplot[mark=none, C2, dashdotted, very thick, domain=280:290] table[y={Testing_accuracy_exploitation}]{results/protonet_miniImageNet.csv};
%                     \addplot[mark=none, C3, solid, very thick, domain=280:290] table[y={Testing_accuracy_tow}]{results/protonet_miniImageNet.csv};
%                 \end{axis}

%                 \draw [] (c1) -- (ax2.north west);
%                 \draw [] (c2) -- (ax2.south east);
%             \end{tikzpicture}
%             \caption{}
%             \label{fig:protonet_miniImageNet_testing_accuracy}
%         \end{subfigure}
%         \hfill\\

%         \begin{subfigure}{0.45 \linewidth}
%             \centering
%             \begin{tikzpicture}
%                 \begin{axis}[
%                     height=0.6 \linewidth,
%                     width=0.8 \linewidth,
%                     xbar=0pt,
%                     % ymin=0,
%                     % ymax=4,
%                     title={Protonet tested on \(15,504\) mini-ImageNet tasks},
%                     % title style={font=\small},
%                     % legend style={at={(0.5,-0.2)},
%                     % legend style={draw=none, font=\small, /tikz/every even column/.append style={column sep=0.5em}, anchor=north, legend columns=2},
%                     % legend pos=north west,
%                     % legend image post style={scale=0.75},
%                     % legend cell align={left},
%                     % ylabel={Prediction accuracy (\%)},
%                     % ylabel={\vphantom{h}},
%                     % ylabel style={font=\small},
%                     % yticklabel style = {font=\small},
%                     symbolic y coords={Uniform,Exploration,Exploitation,TOW},
%                     % xtick=data,
%                     % xticklabel style = {font=\small},
%                     xlabel={Prediction accuracy (\%)},
%                     scale only axis,
%                     enlarge y limits=0.2,
%                     % nodes near coords,
%                     % nodes near coords align={vertical},
%                     bar width = 10pt
%                 ]
%                     \addplot[style={fill=C0, draw=none, yshift=15pt}, error bars/.cd, x dir=both, x explicit] coordinates {
%                         (41.78,Uniform) +- (1.1, 0)
%                     };
%                     \addplot[style={fill=C1, draw=none, yshift=5pt}, error bars/.cd, x dir=both, x explicit] coordinates {
%                         (41.37,Exploration) +- (1.1, 0)
%                     };
%                     \addplot[style={fill=C2, draw=none, yshift=-5pt}, error bars/.cd, x dir=both, x explicit] coordinates {
%                         (41.92,Exploitation) +- (1.1, 0)
%                     };
%                     \addplot[style={fill=C3, draw=none, yshift=-15pt}, error bars/.cd, x dir=both, x explicit] coordinates {
%                         (43.67,TOW) +- (0.9, 0)
%                     };
%                 \end{axis}
%             \end{tikzpicture}
%             \caption{}
%             \label{fig:protonet_miniImageNet_results}
%         \end{subfigure}
%         \caption{EWMA smoothed by a factor 0.05 for Protonet evaluated on mini-ImageNet shows that TOW out-performs the three baselines by a large margin. The error bars denotes the 95 percent confident intervals.}
%         \label{fig:protonet_miniImageNet}
%     \end{figure}
